# Supplementary material for: LP++: A Surprisingly Strong Linear Probe for Few-Shot CLIP
Source: arXiv:2404.02285 source file (2024-04-02)
Supplement: Supplementary file 1 [file X_suppl.tex]

\clearpage
\setcounter{page}{1}
\maketitlesupplementary

\subsection{The upper bound for learning rate}
\label{sec:lr}
In this paper, we consider the cross-entropy loss function $L_{\textrm{CE}}$ as follows,
\begin{equation}
    L_{\textrm{CE}} = -\frac{1}{N}\sum_{i=1}^N\sum_{k=1}^{K}y_{ik}\log\textrm{softmax}(\bm{f}_{i}^{\top}\bm{V}_{k} + \alpha_k \bm{f}_{i}^{\top}\bm{T}_{k})
\label{eq:CE}    
\end{equation}
where $y_{ik}$ is the one-hot encoding of the target $\bm{y}_{i}\in\mathbb{R}^{K}$ with $K$ being the number of classes. 

The upper bound for the learning rate can be found as follows.

Before we dive into the details, we first review some related knowledge. For a convex differentiable function $f$ that has a Lipschitz gradient, we have $\forall \vx,\vz \in \R^N$,
\begin{equation}
    f(\vx) \leq f(\vz) + \nabla f(\vz)^\top(\vx-\vz) + \frac{L}{2} || \vx-\vz ||^2
\end{equation}
with $L > 0$ being the Lipschitz constant. Considering the surrogate function $g(\vx,\vx^i)$ that majorizes the function $f$ at $\vx^i$, i.e., $g(\vx^i,\vx^i)=f(\vx^i)$ and $g(\vx,\vx^i) \geq f(\vx^i)$ hold $\forall \vx$, 
\begin{equation}
    g(\vx,\vx^i) = f(\vx^i) + \nabla f(\vx^i)^\top(\vx-\vx^i) + \frac{L}{2} || \vx-\vx^i ||^2
\end{equation}
and its derivative is
\begin{equation}
     \frac{\partial g(\vx, \vx^i)}{\partial \vx} = \nabla f(\vx^i) + L(\vx-\vx^i).
\end{equation}
We can solve for $\frac{\partial g(\vx, \vx^i)}{\partial \vx}=0$ at
\begin{equation}
     \vx = \vx^i - \frac{1}{L}\nabla f(\vx^i)
\end{equation}
which leads to the update rule,
\begin{equation}
     \vx^{i+1} = \vx^i - \frac{1}{L}\nabla f(\vx^i)
\label{eq:update}     
\end{equation}
where $\eta = \frac{1}{L}$ is the learning rate.

For a twice differentiable function $f$, if there exists $L < \infty$, its hessian matrix has a bounded spectral norm,
\begin{equation}
    || \nabla^2 f(\vx) || \leq L , \forall \vx \in \R^N    
\label{eq:Lipineq}
\end{equation}
So Lipschitz constant $L$ is an upper bound for the largest eigenvalue $\lambda_{\max}$ of the Hessian matrix $\nabla^2 f(\vx)$.

In our case, following \cite{boudiaf2020unifying} with $p_{ik}=\frac{\exp(\bm{f}_{i}^{\top}\bm{V}_{k} + \alpha_k \bm{f}_{i}^{\top}\bm{T}_{k})}{\sum_{j=1}^{K}\exp (\bm{f}_{i}^{\top}\bm{V}_{j} + \alpha_j \bm{f}_{i}^{\top}\bm{T}_{j})}$, the Hessian matrix $\bm{A}_{k}$ of  Eq.~\ref{eq:CE} with respect to $\bm{V}_{k}$ is,
\begin{equation}
    \bm{A}_{k} = \frac{\partial^{2} L_{\textrm{CE}}}{\partial \bm{V}_{k}^{2}} = \frac{1}{N}\sum_{i=1}^N (p_{ik} - p_{ik}^2) \bm{f}_i \bm{f}_i^\top
\end{equation}
In the above equation, the maximum value of $p_{ik} - p_{ik}^2$ is $\frac{1}{4}$ at $p_{ik} = \frac{1}{2}$ and the features $\bm{f}_i$ are normalized, so the trace of matrix $\bm{f}_i \bm{f}_i^\top$ is $||\bm{f}_i||^2 =1$. Since the trace of one matrix is equal to the sum of its eigenvalues, it naturally becomes an upper bound for the largest eigenvalue $\lambda_{\max}^{k}$. Thus we have,
\begin{equation}
    \lambda_{\max}^{k} \leq tr(\bm{A}_{k}) = \sum_{i=1}^N \lambda_{i}^{k} \leq  \frac{1}{N}\sum_{i=1}^N \frac{1}{4} = \frac{1}{4}
\end{equation}
Finally from inequality Eq.~\ref{eq:Lipineq}, we have $\lambda_{\max}^{k} \leq L_{k} = \frac{1}{\eta}$, so the upper bound for the learning rate is,
\begin{equation}
    \eta \leq 4
\end{equation}

\subsection{Derivation of the optimal solution for CE loss}
Following the definition of the output logits mentioned above, the loss of CE is now considered as a function of two sought parameters $\bm{V} = \{\bm{V}_{k}\}_{1\leq k \leq K}$ and $\bm{\alpha} = \{\alpha_{k}\}_{1 \leq k \leq K}$ as follows,
\begin{align}
    L_{\textrm{CE}} &= -\frac{1}{N}\sum_{i=1}^{N}\sum_{k=1}^{K} y_{ik}\log\textrm{softmax}(\bm{f}_{i}^{\top}\bm{V}_{k} + \alpha_k \bm{f}_{i}^{\top}\bm{T}_{k}) \\
    &= g_{1}(\bm{V},\bm{\alpha})+ g_{2}(\bm{V},\bm{\alpha}) 
\end{align}
where $y_{ik}$ is the one-hot encoding of the target $\bm{y}_{i}\in\mathbb{R}^{K}$ with $K$ being the number of classes and $N$ is the number of samples and 
\begin{align}
\scriptsize
         g_{1}(\bm{V},\bm{\alpha}) &= -\frac{1}{N}\sum_{i=1}^N\sum_{k=1}^{K}y_{ik}(\bm{f}_{i}^{\top}\bm{V}_{k} + \alpha_k\bm{f}_{i}^{\top}\bm{T}_{k})\nonumber \\
         &+\frac{\lambda}{2}\sum_{k=1}^{K}(\bm{V}_{k} + \alpha_k\bm{T}_{k})^\top(\bm{V}_{k} + \alpha_k\bm{T}_{k}) \\
     g_{2}(\bm{V},\bm{\alpha}) &= \frac{1}{N}\sum_{i=1}^{N}\log (\sum_{j=1}^{K}\exp(\bm{f}_{i}^{\top}\bm{V}_{j} + \alpha_j\bm{f}_{i}^{\top}\bm{T}_{j})) \nonumber \\
     &-\frac{\lambda}{2}\sum_{k=1}^{K}(\bm{V}_{k} + \alpha_k\bm{T}_{k})^\top(\bm{V}_{k} + \alpha_k\bm{T}_{k})
\end{align}
Note that $g_{1}(\bm{V},\bm{\alpha})$ is a convex function of $\bm{V}_{k}$ and $\alpha_{k}, \forall 1\leq k \leq K$ respectively for all $\lambda$. As for $g_{2}$, we can ensure $g_{2}(\bm{V},\bm{\alpha})$ is also a convex function of these parameters under certain scenarios. To be specific, we set 
\begin{align}
\lambda=\min_{k,l} \sigma_{l}(\bm{A}_{k})    
\end{align}
where $\bm{A}_{k} = \frac{1}{N}\sum_{i=1}^N (p_{ik} - p_{ik}^2) \bm{f}_i \bm{f}_i^\top$ with $p_{ik} = \frac{\exp(\bm{f}_{i}^{\top}\bm{V}_{k} + \alpha_k\bm{f}_{i}^{\top}\bm{T}_{k})}{\sum_{j=1}^{K}\exp(\bm{f}_{i}^{\top}\bm{V}_{j} + \alpha_j\bm{f}_{i}^{\top}\bm{T}_{j})}$ and $\sigma_{l}(\bm{A}_{k})$ is the $l^\textrm{th}$ eigenvalue of $\bm{A}_{k}$. 

\begin{prop}
The optimal solution of $\bm{V}_{k}$ is close to the mean of features of each class when finetuning CE loss function.
\end{prop}

To find the optimal solution of $\bm{V}$, we take derivative of $g_{1}(\bm{V},\bm{\alpha})$ and $g_{2}(\bm{V},\bm{\alpha})$ with respect to $\bm{V}_{k}$ respectively.
\begin{align}
    & \frac{\partial g_{1}(\bm{V},\bm{\alpha})}{\partial\bm{V}_{k}}=-\frac{1}{N}\sum_{i=1}^{N}y_{ik}\bm{f}_{i}+\lambda(\bm{V}_{k} + \alpha_k\bm{T}_{k})\\
    & \frac{\partial g_{2}(\bm{V},\bm{\alpha})}{\partial\bm{V}_{k}}=\frac{1}{N}\sum_{i=1}^{N}\frac{\exp(\bm{f}_{i}^{\top}\bm{V}_{k} + \alpha_k\bm{f}_{i}^{\top}\bm{T}_{k})}{\sum_{j=1}^{K}\exp(\bm{f}_{i}^{\top}\bm{V}_{j} + \alpha_j\bm{f}_{i}^{\top}\bm{T}_{j})}\bm{f}_{i}-\lambda(\bm{V}_{k} + \alpha_k\bm{T}_{k})
\end{align}
Let it be equal to 0, we obtain that $\forall 1\leq k \leq K$, the optimal $\bm{V}_{k}$ for $g_{1}(\bm{V},\bm{\alpha})$ is,
\begin{align}
\bm{V}_{k}^{g_{1}*} & = \frac{1}{\lambda N} \sum_{i=1}^{N}y_{ik}\bm{f}_{i}-\alpha_k\bm{T}_{k}\\
& = \frac{1}{\lambda N} \sum_{i:\bm{y}_{i}=k}\bm{f}_{i}-\alpha_k\bm{T}_{k}\propto \bm{c}_{k} = \frac{1}{|\mathcal{S}_{k}|} \sum_{i:\bm{y}_{i}=k}\bm{f}_{i}
\end{align}
where $\bm{c}_{k}$ is the hard mean of features of class $k$ and $|\mathcal{S}_{k}|$ is the sample size of training set belongs to class $k$.

Similarly, the optimal $\bm{V}_{k}$ for $g_{2}(\bm{V},\bm{\alpha})$ is,
\begin{align}
\bm{V}_{k}^{g_{2}*} & = \frac{1}{\lambda N} \sum_{i=1}^{N}\frac{\exp(\bm{f}_{i}^{\top}\bm{V}_{k} + \alpha_k\bm{f}_{i}^{\top}\bm{T}_{k})}{\sum_{j=1}^{K}\exp(\bm{f}_{i}^{\top}\bm{V}_{j} + \alpha_j\bm{f}_{i}^{\top}\bm{T}_{j})} \bm{f}_{i}-\alpha_k\bm{T}_{k} \\
& \propto \bm{c}_{k}^{s} = \frac{1}{N} \sum_{i=1}^{N}\frac{\exp(\bm{f}_{i}^{\top}\bm{V}_{k} + \alpha_k\bm{f}_{i}^{\top}\bm{T}_{k})}{\sum_{j=1}^{K}\exp(\bm{f}_{i}^{\top}\bm{V}_{j} + \alpha_j\bm{f}_{i}^{\top}\bm{T}_{j})}\bm{f}_{i}
\end{align}
where $\bm{c}_{k}^{s}$ is the soft mean of features of class $k$.

\begin{prop}
The optimal solution of $\alpha_{k}$ is close to the multiplication of features and text weights of each class when finetuning CE loss function.
\end{prop}
To find the optimal solution of $\bm{\alpha}$, we take derivative of $g_{1}(\bm{V},\bm{\alpha})$ and $g_{2}(\bm{V},\bm{\alpha})$ with respect to $\alpha_{k}$ respectively.
\begin{align}
    & \frac{\partial g_{1}(\bm{V},\bm{\alpha})}{\partial\alpha_{k}}=-\frac{1}{N}\sum_{i=1}^{N}y_{ik}\bm{f}_{i}^\top\bm{T}_{k} +\lambda(\bm{V}_{k} + \alpha_k\bm{T}_{k})^\top\bm{T}_{k}\\
    & \frac{\partial g_{2}(\bm{V},\bm{\alpha})}{\partial\alpha_{k}} \nonumber\\
    &=\frac{1}{N}\sum_{i=1}^{N}\frac{\exp(\bm{f}_{i}^{\top}\bm{V}_{k} + \alpha_k\bm{f}_{i}^{\top}\bm{T}_{k})}{\sum_{j=1}^{K}\exp(\bm{f}_{i}^{\top}\bm{V}_{j} + \alpha_j\bm{f}_{i}^{\top}\bm{T}_{j})}\bm{f}_{i}^\top\bm{T}_{k}-\lambda(\bm{V}_{k} + \alpha_k\bm{T}_{k})^\top\bm{T}_{k}
\end{align}
Let it be equal to 0, we obtain that $\forall 1\leq k \leq K$, the optimal $\alpha_{k}$ for $g_{1}(\bm{V},\bm{\alpha})$ is,
\begin{align}
\alpha_{k}^{g_{1}*} & = \frac{1}{\bm{T}_{k}^\top\bm{T}_{k}}\left(\frac{1}{\lambda N} \sum_{i=1}^{N}y_{ik}\bm{f}_{i}^\top\bm{T}_{k}-\bm{V}_{k}^\top\bm{T}_{k}\right)\\
& \propto \frac{1}{|\mathcal{S}_{k}|} \sum_{i:\bm{y}_{i}=k}\bm{f}_{i}^\top\bm{T}_{k}
\end{align}
which is the hard mean of the multiplication of the features and the text weights of class $k$ and $|\mathcal{S}_{k}|$ is the sample size of training set belongs to class $k$.

Similarly, the optimal $\alpha_{k}$ for $g_{2}(\bm{V},\bm{\alpha})$ is,
\begin{align}
\alpha_{k}^{g_{2}*} & = \frac{1}{\bm{T}_{k}^\top\bm{T}_{k}}\left(\frac{1}{\lambda N} \sum_{i=1}^{N}\frac{\exp(\bm{f}_{i}^{\top}\bm{V}_{k} + \alpha_k\bm{f}_{i}^{\top}\bm{T}_{k})}{\sum_{j=1}^{K}\exp(\bm{f}_{i}^{\top}\bm{V}_{j} + \alpha_j\bm{f}_{i}^{\top}\bm{T}_{j})} \bm{f}_{i}^\top\bm{T}_{k}-\bm{V}_{k}^{\top}\bm{T}_{k}\right) \\
& \propto \frac{1}{N} \sum_{i=1}^{N}\frac{\exp(\bm{f}_{i}^{\top}\bm{V}_{k} + \alpha_k\bm{f}_{i}^{\top}\bm{T}_{k})}{\sum_{j=1}^{K}\exp(\bm{f}_{i}^{\top}\bm{V}_{j} + \alpha_j\bm{f}_{i}^{\top}\bm{T}_{j})}\bm{f}_{i}^\top\bm{T}_{k}
\end{align}
which is the soft mean of the multiplication of the features and the text weights of class $k$.

\subsection{Ablation Study}
\subsubsection{Numerical Results on 11 benchmarks}
\begin{table*}[ht]
\footnotesize

\centering
\begin{tabular}{lcccccc}
\hline
\textbf{Number of shots ($k$)} & \textbf{1} & \textbf{2} & \textbf{4} & \textbf{8} & \textbf{16}\\
\hline
\hline
Zero-shot CLIP\cite{radford2021clip} & \multicolumn{5}{c}{60.35}\\
\midrule
LP\cite{radford2021clip} & 22.21 (0.31)  &  31.96 (0.25)  &  41.48 (0.25)  &  49.49 (0.16)  & 56.04 (0.13)  \\
\hline
CoOp$_\text{ IJCV'22}$\cite{Zhou2022coop} & $61.19 \pm 0.17$ & $61.58 \pm 0.40$  &  $62.22 \pm 0.22$  & $62.87 \pm 0.21$  &  $63.70 \pm 0.13$ \\
\hline
%Tip-Adapter\cite{zhang2022tip} & $60.48\pm0.08$ & $60.56\pm0.16$ & $61.02\pm0.12$ & $61.24\pm0.08$ & $61.59\pm0.10$ \\
%\hline
Tip-Adapter-F*\cite{zhang2022tip} & $60.59 \pm0.14$ & $61.42 \pm0.05$ & $62.12 \pm0.06$  & $63.41\pm 0.07$  & $65.06\pm 0.04$ \\
\hline
Tip-Adapter-F*[g] & $61.09 \pm0.22$ & $61.76 \pm0.16$ & $\textbf{62.64} \pm0.09$ & $63.85\pm 0.18$ & $64.98\pm 0.12$ \\ %\textcolor{blue}{(-0.48)} 
\hline
PLOT\cite{chen2023plot} & $60.46 \pm 0.34$ &  $60.73 \pm 0.60$ &  $61.79 \pm 0.39$  &  $62.48 \pm 0.32$ & $63.08 \pm 0.26$  \\
\hline
KgCoOp\cite{Yao2023kgcoop} & $60.90 \pm 0.16$ & $61.44 \pm 0.15$ & $62.00 \pm 0.11$ &$62.20 \pm 0.15$ & $62.43 \pm 0.11$ \\
\hline
ProGrad\cite{Zhu2023prograd} & $\textbf{61.58} \pm 0.27$ & $\textbf{62.14} \pm 0.13$ & $62.59 \pm 0.09$ & $63.04 \pm 0.11$ & $63.54 \pm 0.18$\\
\midrule
\cellcolor{blue!15}{LP++} & \cellcolor{blue!15}{$61.16 \pm 0.14$} & \cellcolor{blue!15}{$61.58 \pm 0.08$} & \cellcolor{blue!15}{$\textbf{62.64} \pm 0.17$} & \cellcolor{blue!15}{$\textbf{63.88} \pm 0.12$} & \cellcolor{blue!15}{$\textbf{65.08} \pm 0.06$}\\
\bottomrule
\end{tabular}
\vspace{0.1cm}
\caption{\textbf{Comparison to state-of-the-art methods.} Classification accuracy (\%) on the ImageNet test set, %averaged over the 11 classification benchmarks, 
with standard derivation over 10 test episodes on ImageNet for different approaches. Best values are highlighted in bold.}% with quantitative values.}
\label{table:resultOther_Imagenet}
\end{table*}

\subsubsection{Domain shift}
To examine the generalization of LP++, we conduct experiments under different distribution shifts. Considering ImageNet as the source data set, we adapt the learnt model on two different target data sets. ImageNet-V2 \cite{Recht2019imagenetv2} and ImageNet-Sketch \cite{Wang2019imagenetsketch} are two variants of ImageNet containing equivalent number of classes as ImageNet but exhibiting significant semantic gaps. \cref{table:resultOther_Imagenet_domainshift} represents the results training each few-shot CLIP method in 16 shot setting and evaluating on the whole test set of the data sets. As shown in the table, LP++ has nearly 10-15\% improvement over LP. LP++ and Tip-Adapter-F achieve better results than prompt learning methods in most cases with LP++ being faster. 

\begin{table}[H]
\footnotesize
\setlength{\tabcolsep}{4pt} % Default value: 6pt

\centering
\begin{tabular}{ccccccc}
\hline
 & ImageNet & -V2 & -Sketch \\
\hline
\hline
Zero-shot CLIP\cite{radford2021clip} & \multicolumn{3}{c}{60.35}\\
\hline
LP\cite{radford2021clip} & $56.04 \pm 0.13$  &  $45.76 \pm 0.24$  &  $19.94 \pm 0.27$   \\
\hline
CoOp\cite{Zhou2022coop} & $63.70 \pm 0.13$ & $55.97 \pm 0.10$ & $33.89 \pm 0.57$ \\
\hline
%Tip-Adapter\cite{zhang2022tip} & $61.59 \pm 0.10$ & $52.70 \pm 0.10$ & $34.14 \pm 0.10$\\
%\hline
Tip-Adapter-F*\cite{zhang2022tip} & $65.07 \pm 0.04$ & $\textbf{56.45} \pm 0.08$ & $34.43 \pm 0.12$ \\
\hline
Tip-Adapter-F*[g]\cite{zhang2022tip} & $64.98 \pm 0.12$ & $54.76 \pm 0.19$ & $32.82 \pm 0.40$ \\
\hline
PLOT\cite{chen2023plot} & $63.08 \pm 0.26$ & $54.09 \pm 0.39$& $32.57 \pm 0.76$ \\
\hline
KgCoOp\cite{Yao2023kgcoop} & $62.43 \pm 0.11$ & $54.70 \pm 0.24$ & $\textbf{35.16} \pm 0.12$ \\
\hline
ProGrad\cite{Zhu2023prograd} & $63.54 \pm 0.18$ & $55.76 \pm 0.28$ & $34.50 \pm 0.31$  \\
\hline
 LP++ & $\textbf{65.08} \pm 0.06$ & $56.22 \pm 0.10$ & $34.45 \pm 0.19$\\
\hline
\end{tabular}
\vspace{0.05cm}
\caption{\footnotesize Averaged classification accuracy (\%) with standard derivation over 10 episodes on robustness to domain shift of ImageNet data set with 16 shots of different models with quantitative values.}
\label{table:resultOther_Imagenet_domainshift}
\end{table}
